# Supplementary material for: OntoSeer -- A Recommendation System to Improve the Quality of Ontologies
Source: arXiv:2202.02125 source file (2022-02-04)
Supplement: Supplementary file 1 [file Appendix.tex]

\section*{Appendix}

The survey questions that were asked to the users are listed below.

\begin{enumerate}
    \item 
        How experienced are you with Ontology Modelling?
    \item
    How experienced are you with using Prot\'eg\'e?
    \item
      Do you know about LOV and ontology repositories such as BioPortal?
    \item
    If Yes, please specify how often do you reuse classes and properties from LOV and ontology repositories?
    \item 
    Do you use Ontology Design Patterns (ODPs) while modelling?
    \item
        If Yes, please specify how often do you use ODPs?
    \item
        How was the installation process?
    \item
        This section should be answered if competency questions have been provided to OntoSeer.
        \begin{enumerate}
        \item
            How useful are the class and property recommendations?
        \item
            How useful are the Ontology vocabulary recommendations?
        \item
            How useful are the ODP recommendations?
        \item
            How useful are the axiom recommendations?
        \item
  
        \end{enumerate}
    \item This section should be answered if competency questions are not provided to OntoSeer.
        \begin{enumerate}
            \item How useful are the Ontology vocabulary recommendations?
            \item How useful are the ODP recommendations?
            \item How useful are the axiom recommendations?
        
        \end{enumerate}
    \item How was your experience of modelling an ontology without OntoSeer?
    \item How was your experience of modelling an ontology with OntoSeer?
    \item Does Ontoseer help in saving modelling time? 
    \item Do you have any suggestions for improving the user experience?
\end{enumerate}
